# Supplementary material for: Empirical Frequentist Coverage of Deep Learning Uncertainty Quantification Procedures
Source: arXiv:2010.03039 source file (2021-02-24)
Supplement: Supplementary file 1 [file appendix.pdf]

# A Appendix

## A.1 Regression Tables

| Dataset — Method | Linear Regression | GP | Ensemble | Dropout | LL Dropout | SVI | LL SVI |
|---|---|---|---|---|---|---|---|
| Boston Housing | 0.9461 (5.61e-03) | **0.9765 (5.05e-03)** | 0.5912 (1.43e-02) | 0.602 (1.64e-02) | 0.1902 (2.01e-02) | 0.9434 (6.04e-03) | 0.9339 (8.48e-03) |
| Concrete | 0.9437 (2.68e-03) | **0.967 (3.02e-03)** | 0.5854 (1.04e-02) | 0.7282 (1.17e-02) | 0.0932 (1.75e-02) | 0.9581 (3.61e-03) | 0.9443 (6.72e-03) |
| Energy | 0.8957 (4.66e-03) | 0.8857 (6.96e-03) | 0.8669 (5.26e-03) | 0.8013 (2.00e-02) | 0.2597 (2.75e-02) | 0.9773 (3.02e-03) | **0.9938 (2.99e-03)** |
| Kin8nm | 0.9514 (1.20e-03) | **0.9705 (1.53e-03)** | 0.6706 (4.43e-03) | 0.8037 (8.15e-03) | 0.1984 (1.36e-02) | 0.9618 (2.63e-03) | 0.9633 (1.36e-03) |
| Naval Propulsion Plant | 0.9373 (1.59e-03) | **0.9994 (2.12e-04)** | 0.8036 (5.99e-03) | 0.9212 (6.76e-03) | 0.2683 (2.51e-02) | 0.9797 (1.88e-03) | 0.9941 (1.25e-03) |
| Power Plant | **0.9646 (1.14e-03)** | 0.9614 (1.26e-03) | 0.4008 (1.12e-02) | 0.432 (1.47e-02) | 0.1138 (1.41e-02) | 0.9626 (1.13e-03) | 0.9623 (1.60e-03) |
| Protein Tertiary Structure | **0.9619 (4.71e-04)** | 0.959 (4.72E-04) | 0.4125 (2.98e-03) | 0.3846 (1.36e-02) | 0.1182 (1.35e-02) | 0.9609 (2.27e-03) | 0.9559 (1.72e-03) |
| Wine Quality Red | 0.9425 (2.32e-03) | **0.9472 (3.28e-03)** | 0.3919 (1.18e-02) | 0.3566 (1.83e-02) | 0.1616 (7.45e-03) | 0.9059 (8.19e-03) | 0.8647 (8.77e-03) |
| Yacht Hydrodynamics | 0.9449 (7.86e-03) | 0.9726 (6.73e-03) | 0.9161 (7.38e-03) | 0.3871 (2.82e-02) | 0.2081 (2.54e-02) | 0.9807 (6.97e-03) | **0.9899 (6.03e-03)** |

Table A1: The average coverage of six methods across nine datasets with the standard error over 20 cross validation folds in parentheses.

| Dataset — Method | Linear Regression | GP | Ensemble | Dropout | LL Dropout | SVI | LL SVI |
|---|---|---|---|---|---|---|---|
| Boston Housing | 2.0424 (6.87E-03) | 1.8716 (1.17E-02) | 0.4432 (7.82E-03) | 0.6882 (2.19E-02) | 0.1855 (2.05E-02) | 1.301 (2.56E-02) | 1.148 (2.36E-02) |
| Concrete | 2.4562 (2.22E-03) | 2 (3.32E-03) | 0.4776 (9.03E-03) | 1.0342 (1.79E-02) | 0.1028 (2.04E-02) | 1.5116 (1.72E-02) | 1.2293 (1.41E-02) |
| Energy | 1.144 (2.29E-03) | 1.0773 (2.64E-03) | 0.2394 (2.56E-03) | 0.5928 (1.22E-02) | 0.1417 (1.61E-02) | 0.8426 (1.73E-02) | 0.7974 (1.95E-02) |
| Kin8nm | 3.0039 (9.76E-04) | 2.3795 (7.02E-03) | 0.5493 (2.37E-03) | 1.2355 (1.37E-02) | 0.2024 (1.22E-02) | 1.6697 (7.75E-03) | 1.2624 (2.99E-03) |
| Naval Propulsion Plant | 1.5551 (7.12E-04) | 0.3403 (1.00E-02) | 0.6048 (4.86E-03) | 1.1593 (6.45E-03) | 0.2281 (1.83E-02) | 1.3064 (1.38E-01) | 0.488 (5.44E-03) |
| Power Plant | 1.0475 (7.09E-04) | 0.9768 (9.63E-04) | 0.2494 (6.72E-03) | 0.3385 (1.69E-02) | 0.0918 (9.06E-03) | 1.0035 (1.88E-03) | 0.9818 (3.64E-03) |
| Protein Tertiary Structure | 3.3182 (3.21E-04) | 3.2123 (3.47E-03) | 0.6804 (3.77E-03) | 0.9144 (1.41E-02) | 0.3454 (1.99E-02) | 2.9535 (3.82E-02) | 2.6506 (2.20E-02) |
| Wine Quality Red | 3.1573 (1.82E-03) | 3.1629 (4.07E-03) | 0.7763 (1.31E-02) | 0.7841 (2.91E-02) | 0.3481 (1.61E-02) | 2.7469 (2.72E-02) | 2.3597 (2.70E-02) |
| Yacht Hydrodynamics | 2.3636 (2.89E-03) | 1.6974 (7.57E-03) | 0.4475 (9.76E-03) | 0.5443 (2.22E-02) | 0.1081 (9.83E-03) | 0.657 (3.54E-02) | 0.69 (3.81E-02) |

Table A2: The average width of the posterior prediction interval of six methods across nine datasets with the standard error over 20 cross validation folds in parentheses. Width is reported in terms of standard deviations of the response variable in the training set.

## A.2 Classification Results

| Method | Mean Test Set Coverage (SE) | Mean Test Set Width (SE) | Mean Rotation Shift Coverage (SE) | Mean Rotation Shift Width (SE) | Mean Translation Shift Coverage (SE) | Mean Translation Shift Width (SE) |
|---|---|---|---|---|---|---|
| Dropout | 0.9987 (6.32E-05) | 1.06 (1.38E-04) | 0.5519 (2.91E-02) | 2.3279 (6.64E-02) | 0.5333 (3.54E-02) | 2.3527 (6.34E-02) |
| Ensemble | 0.9984 (7.07E-05) | 1.0424 (2.07E-04) | 0.5157 (3.11E-02) | 2.0892 (5.44E-02) | 0.5424 (3.33E-02) | 2.3276 (6.66E-02) |
| LL Dropout | 0.9985 (1.05E-04) | 1.0561 (1.89E-03) | 0.552 (2.93E-02) | 2.3162 (6.73E-02) | 0.5388 (3.52E-02) | 2.3658 (6.66E-02) |
| LL SVI | 0.9984 (1.14E-04) | 1.0637 (1.65E-03) | 0.5746 (2.77E-02) | 2.6324 (8.41E-02) | 0.535 (3.51E-02) | 2.3294 (6.46E-02) |
| SVI | 0.9997 (7.35E-05) | 1.5492 (2.19E-02) | 0.7148 (2.06E-02) | 4.8549 (1.44E-01) | 0.754 (1.96E-02) | 5.6803 (1.99E-01) |
| Temp scaling | 0.9986 (1.36E-04) | 1.0642 (1.98E-03) | 0.5243 (3.10E-02) | 2.2683 (6.17E-02) | 0.5375 (3.33E-02) | 2.347 (6.21E-02) |
| Vanilla | 0.9972 (1.16E-04) | 1.032 (9.06E-04) | 0.4715 (3.28E-02) | 1.7492 (3.78E-02) | 0.4798 (3.50E-02) | 1.801 (3.84E-02) |

Table A3: MNIST average coverage and width for the test set, rotation shift, and translation shift.

| Method | Mean Test Set Coverage (SE) | Mean Test Set Width (SE) | Mean Translation Shift Coverage (SE) | Mean Translation Shift Width (SE) |
|---|---|---|---|---|
| Dropout | 0.9883 (3.79E-04) | 1.5778 (2.68E-03) | 0.9696 (2.48E-03) | 2.0709 (5.11E-02) |
| Ensemble | 0.9922 (3.08E-04) | 1.4925 (1.52E-03) | 0.9806 (1.65E-03) | 1.9246 (4.49E-02) |
| LL Dropout | 0.9628 (1.40E-03) | 1.3007 (3.99E-03) | 0.9184 (5.59E-03) | 1.6678 (4.16E-02) |
| LL SVI | 0.9677 (1.10E-03) | 1.2585 (2.60E-03) | 0.929 (4.55E-03) | 1.5044 (2.61E-02) |
| SVI | 0.9789 (6.41E-04) | 1.5579 (6.31E-03) | 0.9543 (2.89E-03) | 1.9286 (3.69E-02) |
| Temp scaling | 0.9871 (3.51E-04) | 1.5987 (1.19E-02) | 0.9707 (1.97E-03) | 2.1266 (5.30E-02) |
| Vanilla | 0.9686 (6.06E-04) | 1.2611 (3.90E-03) | 0.9296 (4.36E-03) | 1.5064 (2.58E-02) |

Table A4: CIFAR-10 average coverage and width for the test set and translation shift.

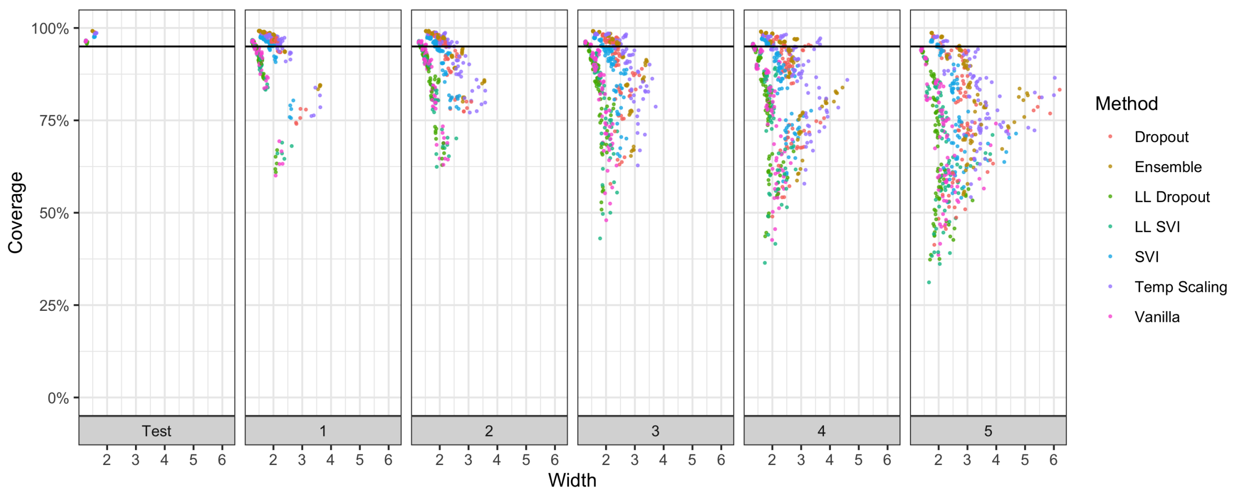


Figure 7: (reproduced from Figure 7 of the main text for clarity) 0The effect of corruption intensity on coverage levels vs. width in CIFAR-10-C. Each facet panel represents a different corruption level, while points are the coverage of a model on one of 16 corruptions. Each facet has 80 points per method, since 5 iterations were trained per method. For methods with points at the same coverage level, the superior method is to the left as it has a lower width.

| Method | Mean Test Set Coverage (SE) | Mean Test Set Width (SE) | Mean Corruption Coverage (SE) | Mean Corruption Width (SE) |
|---|---|---|---|---|
| Dropout | 0.987 (3.72E-04) | 1.578 (2.68E-03) | 0.886 (6.34E-03) | 2.313 (3.03E-02) |
| Ensemble | 0.992 (9.70E-05) | 1.492 (1.52E-03) | 0.911 (5.16E-03) | 2.425 (3.69E-02) |
| LL Dropout | 0.960 (8.77E-04) | 1.301 (3.99E-03) | 0.815 (7.48E-03) | 1.699 (1.53E-02) |
| LL SVI | 0.964 (6.64E-04) | 1.258 (2.60E-03) | 0.817 (7.52E-03) | 1.781 (2.15E-02) |
| SVI | 0.976 (5.10E-04) | 1.558 (6.31E-03) | 0.881 (5.45E-03) | 2.161 (2.32E-02) |
| Temp Scaling | 0.985 (4.54E-04) | 1.599 (1.19E-02) | 0.899 (4.85E-03) | 2.636 (3.86E-02) |
| Vanilla | 0.964 (6.36E-04) | 1.261(3.90E-03) | 0.823 (7.10E-03) | 1.790 (2.16E-02) |

Table A5: The mean coverage and widths on the test set of CIFAR-10 as well as on the mean coverage and width averaged over 16 corruptions and 5 intensities.

| Method | Mean Test Set Coverage | Mean Test Set Width | Mean Corruption Coverage (SE) | Mean Corruption Width (SE) |
|---|---|---|---|---|
| Dropout | 0.9613 | 13.2699 | 0.8579 (1.61E-02) | 87.5784 (7.80E+00) |
| Ensemble | 0.9701 | 13.0613 | 0.9231 (7.13E-03) | 105.3608 (8.57E+00) |
| LL Dropout | 0.9552 | 10.7707 | 0.8688 (1.18E-02) | 88.0326 (8.04E+00) |
| LL SVI | 0.9327 | 10.5624 | 0.777 (1.76E-02) | 65.9982 (5.01E+00) |
| Temp Scaling | 0.9613 | 15.4811 | 0.8829 (1.10E-02) | 105.1409 (8.43E+00) |
| Vanilla | 0.9525 | 11.0255 | 0.8529 (1.27E-02) | 80.687 (7.16E+00) |

Table A6: The mean coverage and widths on the test set of ImageNet as well as on the mean coverage and width averaged over 16 corruptions and 5 intensities.

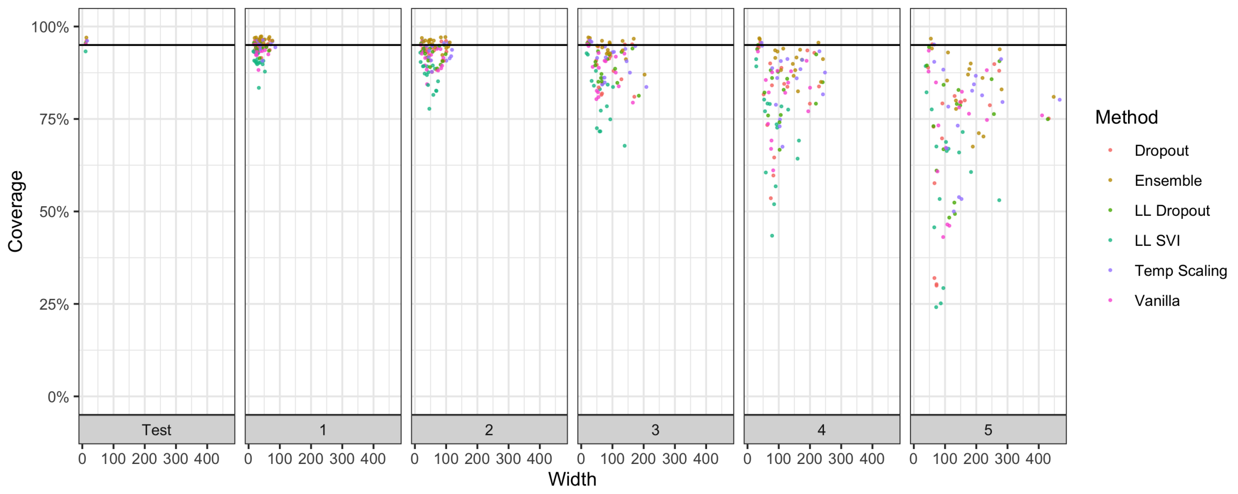


Figure A1: The effect of corruption intensity on coverage levels vs. width in ImageNet-C. Each facet panel represents a different corruption level, while points are the coverage of a model on one of 16 corruptions. Each facet has 16 points per method, as only only 1 iteration was trained per method. For methods equal coverage, the superior method is to the left as it has a lower width.
